# Supplementary material for: Relative Illumination Fields: Learning Medium and Light Independent Underwater Scenes
Source: arXiv:2504.10024 source file (2025-04-14)
Supplement: Supplementary file 1 [file X_suppl.tex]

\clearpage
\setcounter{page}{1}
\maketitlesupplementary

\section{Videos}
\label{sec:video}
The supplementary material contains extended video results for the experiments discussed in the main paper in Fig.4 that show consistent results from many perspectives, both for scene colors as well as for the lights.

\section{Evaluation on Color Charts}
We additionally assess the effectiveness of water removal by comparing to 
Levy et al. \cite{levy2023seathru} based on relative scene
color accuracy, tested on 3 different Jerlov-like tank waters mixed with food colorants and a scattering agent.
For each we capture image sequences with a GoPro Hero9 with attached artificial illumination. Restoration is then evaluated for each water type using a MacBeth chart. 

\begin{table}[ht!]
\centering
\begin{tabular}{lccc}
\toprule
&  Type \texttt{IB} & Type \texttt{II} & Type \texttt{3C} \\
\midrule
Levy \etal \cite{levy2023seathru}
 & \textbf{5.71} &  5.83 & 7.76\\
\midrule
Proposed
 & 11.70 & \textbf{ 3.72} & \textbf{5.36}\\
\end{tabular}
\caption{Evaluation of water removal performance using a Macbeth chart based method, reporting angular RGB error in degrees\cite{Finlayson-PAMI-2017}. For both methods, we pre-scale the restored value of the white MacBeth field to the RGB value predicted from spectrophotometer readings of the patch and then transformed into GoPro space.}
\label{tab:color_error_neu}
\end{table}

We report average angular errors from color chart images in the held-out test set not used during training. Test image poses are estimated
using structure-from-motion and the evaluated methods synthesize images from these
poses. With both methods we predict wideband RGB albedo resp. restored images. In order to avoid the error being contaminated by global white balancing effects, we pick the white MacBeth field and compute global factors for R,G and B respectively in both restorations such that the white fields become equal. Afterwards we compute the error of Finlayson et al.\cite{Finlayson-PAMI-2017} with respect to independently obtained spectrophotometer readings projected to GoPro space on all other fields. Note that the implementation of \cite{levy2023seathru} requires 16 bit integers, where we noticed quantization effects during our fusion of input image to a common HDR space. If we reimplemented the interface to float similarly to what our method is using, results for \cite{levy2023seathru} would likely slightly improve. We still believe that the trend in the data will persist that the more turbid/denser waters exibit strong light cones and scattering effects that our method tends to compensate better. Again, please note that \cite{levy2023seathru} is not designed to cope with underwater light cones, but we still find it instructive to compare our method to something.
